# Supplementary material for: Fast Concurrent Data Sketches
Source: arXiv:1902.10995 source file (2019-12-05)
Supplement: Supplementary file 1 [file appendixErrorBounds.tex]

\section{Derivations of error bounds}
\label{sec:appendix-error-bounds}

\subsection{RSE and RSME definition}
\label{ssec:RSE-RMSE}

Given $n$ i.i.d random variable $X_1, \dots , X_n$, the \emph{Relative Standard Error (RSE)}
of some estimate $E=f(X_1, \dots, X_n)$ for some function $f$ with a PDF $f_E(e)$ from some value $\hat{e}$, is defined to be:
\begin{align*}
    \text{RSE}[E]=\sqrt{\Int_{-\infty}^{\infty} \frac{(e-\hat{e})^2}{n^2}} f_E(e) de
\end{align*}

Furthermore, the \emph{Relative Standard Mean Error (RSME)} is the RSE for
$\hat{e}=E[E]$, i.e., the relative standard error from the mean. The RSME
can be expanded to:
\begin{align*}
    \text{RSME}[E]=\sqrt{\Int_{-\infty}^{\infty} \frac{(e-\hat{e})^2}{n^2}} f_E(e) de = \sqrt{\frac{\sigma^2(E)}{n}}
\end{align*}
\subsection{$\Theta$ sketch error bounds}
\label{ssec:theta-error-bounds}

\begin{lemma}
    The RSE of $e_{\mathcal{A}}$ satisfies the inequality $\text{RSE}[e_{\mathcal{A}}] \leq \sqrt{\frac{\sigma^2(e_{\mathcal{A}})}{n^2}} + \sqrt{\frac{(E[e_{\mathcal{A}}] - n)^2}{n^2}}$.
    \label{lemma:theta-adversary-bound}
\end{lemma}
\begin{proof}
    Using the definition given in the full paper~\cite{rinberg2019fast}:%supplementary material Section~\ref{ssec:RSE-RMSE}:
    \begin{align*}
    \begin{split}
    \text{RSE}[e_{\mathcal{A}}]^2 &= \frac{1}{n^2} \Int_{-\infty}^{\infty} (e - n)^2 \cdot f_{e_{\mathcal{A}}}(e) \,de \\
    &= \frac{1}{n^2} \Int_{-\infty}^{\infty} (e - E[e_{\mathcal{A}}] + E[e_{\mathcal{A}}] - n)^2 \cdot f_{e_{\mathcal{A}}}(e) \,de \\
    &\leq \frac{1}{n^2} \Int_{-\infty}^{\infty} \left((e - E[e_{\mathcal{A}}])^2 + (E[e_{\mathcal{A}}] - n)^2 \right)\cdot f_{e_{\mathcal{A}}}(e) \,de \\
    &= \frac{\sigma^2(e_{\mathcal{A}}) + (E[e_{\mathcal{A}}] - n)^2}{n^2} \\
    \text{RSE}[e_{\mathcal{A}}] &\leq \sqrt{\frac{\sigma^2(e_{\mathcal{A}})}{n^2}} + \sqrt{\frac{(E[e_{\mathcal{A}}] - n)^2}{n^2}}
    \end{split}
    \end{align*}
\end{proof}

\begin{claim}
    Consider $j$ values $X_i$, $1 \leq i \leq j$, in the interval $[0,1]$,
    let $M_{(i)}$ be the $i^{th}$ minimum value
    among the $j$. The $X_i$ that maximises $\abs{\frac{k-1}{x}-n}$ for a given $n$
    is either $M_{(0)}$ or $M_{(j)}$.
    \label{claim:max-val}    
\end{claim}
\begin{proof}
    Assume for the sake of contradiction that the variable that
    maximises $\abs{\frac{k-1}{x}-n}$ is $M_{(i)}$ for $0<i<j$.  We consider two cases:
    \begin{itemize}
    \item If $\frac{k-1}{M_{(i)}} \leq n$, as $M_{(j)} > M_{(i)}$ then $\frac{k-1}{M_{(j)}} < \frac{k-1}{M_{(i)}} \leq n$,
    therefore $\abs{\frac{k-1}{M_{(j)}}-n} > \abs{\frac{k-1}{M_{(i)}}-n}$, which is a contradiction.
    \item If $\frac{k-1}{M_{(i)}} > n$, as $M_{(0)} < M_{(i)}$ then $\frac{k-1}{M_{(0)}} > \frac{k-1}{M_{(i)}} > n$,
    therefore $\abs{\frac{k-1}{M_{(0)}}-n} > \abs{\frac{k-1}{M_{(i)}}-n}$, which is a contradiction.
    \end{itemize}
\end{proof}

\paragraph{Computation of $e_{{\mathcal{A}}_s}$ expectation and error} Recall the the ${\mathcal{A}}_s$ knows the oracles coin
flips, therefore knows $M_{(k)}$ and $M_{(k+r)}$, and chooses $M^r_{(k)}$ accordingly. Therefore, we our analysis
is on the order statistics of the full stream, as it is this that the adversary sees. From order statistics, the joint probability density
function of $M_{(k)}, M_{(k+r)}$ is:
\begin{align*}
f_{M_{(k)},M_{(k+r)}}(m_k,m_{k+r}) = n!{m_k^{k-1}\over (k-1)!}{(m_{k+r}-m_k)^{r-1}\over(r-1)!}{(1-m_{k+r})^{n-(k+r)}\over (n-(k+r))!}.
\end{align*}

The expectation of $e_{{\mathcal{A}}_s}$ and $e_{{\mathcal{A}}_s}^2$ can be computed as follows:
\begin{equation}
    \begin{split}
    E[e_{{\mathcal{A}}_s}] = \Int_{0}^{1} \Int_{0}^{m_k} e_{{\mathcal{A}}_s} \cdot f_{M_{(k)},M_{(k+r)}}(m_k,m_{k+r}) \,dm_{k+r}\,dm_k \\
    E[e_{{\mathcal{A}}_s}^2] = \Int_{0}^{1} \Int_{0}^{m_k} \left[e_{{\mathcal{A}}_s} \right] ^2 \cdot f_{M_{(k)},M_{(k+r)}}(m_k,m_{k+r}) \,dm_{k+r}\,dm_k
    \end{split}
    \label{eq:strong-expectation}
\end{equation}
Finally, the RSE of $e_{{\mathcal{A}}_s}$ is derived from the standard error of $e_{{\mathcal{A}}_s}$:
\begin{equation}
    \begin{split}
    \text{RSE}[e_{{\mathcal{A}}_s}]^2 &= \frac{1}{n^2}\Int_{0}^{1} \Int_{0}^{m_k} \left( e_{{\mathcal{A}}_s} - n \right)^2 \cdot f_{M_{(k)},M_{(k+r)}}(m_k,m_{k+r}) \,dm_{k+r}\,dm_k \\
    &= \frac{1}{n^2} \Int_{0}^{1} \Int_{0}^{m_k} \left( e_{{\mathcal{A}}_s} -E[e_{{\mathcal{A}}_s}] + E[e_{{\mathcal{A}}_s}] - n \right)^2 \cdot f_{M_{(k)},M_{(k+r)}}(m_k,m_{k+r}) \,dm_{k+r}\,dm_k \\
    &\leq \frac{1}{n^2} \left(\sigma^2(e_{{\mathcal{A}}_s}) + (e_{{\mathcal{A}}_s} - n)^2 \right)\\
    \text{RSE}[e_{{\mathcal{A}}_s}] &\leq \sqrt{\frac{\sigma^2(e_{{\mathcal{A}}_s}) + (e_{{\mathcal{A}}_s} - n)^2}{n^2}} \\
    &\leq \sqrt{\frac{\sigma^2(e_{{\mathcal{A}}_s})}{n^2}} + \sqrt{\frac{(e_{{\mathcal{A}}_s} - n)^2}{n^2}}
    \end{split}
    \label{eq:strong-se-bound}
\end{equation}

\paragraph{Computation of $e_{{\mathcal{A}}_w}$ expectation and error} Recall that ${\mathcal{A}}_w$ always hides $r$ element smaller than $\Theta$, thus
forcing $M^r_{(k)}=M_{(k+r)}$. Here too our analysis is on the order statistics of the full stream, as this is what the adversary sees.
The expectation of $e_{{\mathcal{A}}_w}$ and $e_{{\mathcal{A}}_w}^2$ is computed using well known equations from order statistics:
\begin{align*}
    E[e_{{\mathcal{A}}_w}]&=E\left[ \frac{k-1}{M_{(k+r)}} \right]=n\frac{k-1}{k+r-1} \\
    E[e_{{\mathcal{A}}_w}^2]&=(k-1)^2\frac{n(n-1)}{(k+r-2)(k+r-1)} \\
    \sigma^2[e_{{\mathcal{A}}_w}] &= E[e_{{\mathcal{A}}_w}^2] - E[e_{{\mathcal{A}}_w}]^2 \\
    &=(k-1)^2\frac{n(n-1)}{(k+r-2)(k+r-1)} - \left(n\frac{k-1}{k+r-1} \right)^2 \\
    &< \frac{n(k-1)^2}{k+r-1}\left[\frac{n}{(k+r-2)(k+r-1)}\right] \\
    \sigma^2[e_{{\mathcal{A}}_w}] &< \frac{n^2}{k+r-2}
\end{align*}

We derive following equation:
\begin{equation}
    \sqrt{\frac{\sigma^2[e_{{\mathcal{A}}_w}]}{E[e_{{\mathcal{A}}_w}]}}<\frac{1}{k-2}
    \label{eq:ss-rse}
\end{equation}

Finally, the RSE of $e_{{\mathcal{A}}_w}$ is derived from the standard error of $e_{{\mathcal{A}}_w}$, and as $E[e_{{\mathcal{A}}_w}] < n$,
and using the same ``trick'' as in Equation~\ref{eq:strong-se-bound}:
\begin{align*}
    \text{RSE}[e_{{\mathcal{A}}_w}]^2 &= \frac{1}{n^2}\Int_{0}^{1} \left( e_{{\mathcal{A}}_w} - n \right)^2 \cdot f_{M_{(k+r)}}(m_{k+r}) \,dm_{k+r} \\
    &< \frac{1}{n^2} \left(\sigma^2(e_{{\mathcal{A}}_w}) + (E[e_{{\mathcal{A}}_w}] - n)^2 \right)\\
    \text{RSE}[e_{{\mathcal{A}}_w}] &< \sqrt{\frac{\sigma^2(e_{{\mathcal{A}}_w})}{E[e_{{\mathcal{A}}_w}]^2}} + \sqrt{\frac{(E[e_{{\mathcal{A}}_w}] - n)^2}{n^2}}
\end{align*}

Using Equation~\ref{eq:ss-rse}:
\begin{equation}
    \text{RSE}[e_{{\mathcal{A}}_w}] < \sqrt{\frac{1}{k-2}} + \frac{r}{k-2}
    \label{eq:theta-rse-weak-bound}
\end{equation}

\subsection{Quantiles sketch error bounds}
\label{ssec:quantiles-sketch-error-bounds}

We begin by analysing the range given in Equation~\ref{eq:rank-range-2} for $0 \leq \phi \leq 0.5$.

\begin{claim}
    For $0 \leq \phi \leq 0.5$ and $i,j>0$ such that $0 \leq i+j \leq r$ and $\epsilon < 0.5$, then: (1) $(1-\phi)i-\phi j + \epsilon(n-(i+j)) \leq (1-\phi) r + \epsilon(n-r)$,
    and (2) $\phi j - (1-\phi)i + \epsilon(n-(i+j)) \leq (1-\phi) r + \epsilon(n-r)$.
    \label{clm:quantiles-bottom-half}
\end{claim}
\begin{proof}
    As $\phi \leq 0.5$, and $\epsilon \ll 0.5$ then $1-\phi-\epsilon > 0$. As $0 \leq i+j \leq r$, then $i \leq r$.
    \begin{align}
        f(i,j)&=(1-\phi)i-\phi j + \epsilon(n-(i+j)) \leq (1-\phi)i + \epsilon(n-i) \leq (1-\phi-\epsilon)i +\epsilon n \\
        &\leq (1-\phi-\epsilon)r +\epsilon n = (1-\phi)r+\epsilon(n-r) = f(r,0)
    \end{align}

    As $\phi \leq 0.5$, then $\phi \leq 1-\phi$, and as As $0 \leq i+j \leq r$, then $i \leq r$
    \begin{align}
        \phi j - (1-\phi)i + \epsilon(n-(i+j)) \leq (1-\phi )j +\epsilon (n-j)  \leq (1-\phi) r + \epsilon (n-r)
    \end{align}
\end{proof}

We next analyse the same range for $0.5 < \phi \leq 1$.

\begin{claim}
    For $0.5 < \phi \leq 1$ and $i,j>0$ such that $0 \leq i+j \leq r$ and $\epsilon < 0.5$, then: (1) $\phi i - (1-\phi)j + \epsilon(n-(i+j)) \leq \phi r + \epsilon(n-r)$, 
    and (2) $(1-\phi)i - \phi j + \epsilon(n-(i+j)) \leq \phi r + \epsilon(n-r)$.
    \label{clm:quantiles-top-half}
\end{claim}
\begin{proof}
    As $\phi > 0.5$, and $\epsilon \ll 0.5$ then $\phi-\epsilon > 0$. As $0 \leq i+j \leq r$, then $i \leq r$.
    \begin{align}
        f(i,j)=\phi i - (1-\phi)j + \epsilon(n-(i+j)) \leq \phi i +\epsilon (n-i) \leq (\phi - \epsilon)i + \epsilon n \leq \phi r + \epsilon(n-r) = f(r,0)
    \end{align}

    As $\phi > 0.5$, then $(1-\phi) \leq \phi$, and as As $0 \leq i+j \leq r$, then $i \leq r$
    \begin{align}
        (1-\phi)i - \phi j + \epsilon(n-(i+j)) \leq \phi i + \epsilon (n-i) \leq \phi r + \epsilon(n-r)
    \end{align}
\end{proof}

Putting the two claims together we get:

\begin{claim}
    For $0 \leq \phi \leq 1$ and $i,j>0$ such that $0 \leq i+j \leq r$ and $\epsilon \ll 0.5$, then: (1) $\phi i - (1-\phi)j + \epsilon(n-(i+j)) \leq r + \epsilon(n-r)$,
    and (2) $(1-\phi)i - \phi j + \epsilon(n-(i+j)) \leq r + \epsilon(n-r)$.
    \label{clm:helper}
\end{claim}
\begin{proof}
    From Claim~\ref{clm:quantiles-bottom-half}, for $0 \leq \phi \leq 0.5$ then both inequalities are bounded by $(1-\phi) r + \epsilon(n-r)$, and as $\phi \geq 0$ then
    $(1-\phi) r + \epsilon(n-r) \leq r + \epsilon(n-r)$.

    From Claim~\ref{clm:quantiles-top-half}, for $0.5 < \phi \leq 1$ then both inequalities are bounded by $\phi r + \epsilon(n-r)$, and as $\phi \leq 1$ then
    $\phi r + \epsilon(n-r) \leq r + \epsilon(n-r)$.
\end{proof}

Finally, we prove a bound on the rank of the element returned. 
\begin{lemma}
    Given parameters $(\epsilon,\delta)$ if $\epsilon<0.5$, then the $r$-relaxed
    quantiles sketch returns an element whose rank is
    between $(\phi-\epsilon_r)n$ and $(\phi+\epsilon_r)n$ with probability at
    least $1-\delta$, where $\epsilon_r=\epsilon - \frac{r \epsilon}{n} + \frac{r}{n}$.
    \label{lemma:quantiles-weak-adversary}
\end{lemma}
\begin{proof}
    Given parameters $(\epsilon,\delta)$, and given that the adversary hides $i$ elements below the
    $\phi$ quantile and $j$ elements above it, such that $0\leq i+j\leq r$, the rank of the element returned
    by the query is in the range given in Equation~\ref{eq:rank-range-2} w.p. at least $1-\delta$:
    \begin{align*}
        \left[\phi n - (\phi j - (1-\phi)i+\epsilon(n-(i+j))), \phi n + ((1-\phi)i - \phi j +\epsilon(n-(i+j))) \right].
    \end{align*}

    From Claim~\ref{clm:helper}, this range is contained within the range:
    \begin{align*}
        \left[\phi n - (r + \epsilon(n-r)), \phi n + (r + \epsilon(n-r)) \right].
    \end{align*}
    Which can be rewritten as the range $\left(\phi \pm \left(\epsilon - \frac{r \epsilon}{n} + \frac{r}{n}\right)\right)n$.
    Meaning the rank of the element returned is between $(\phi-\epsilon_r)n$ and $(\phi+\epsilon_r)n$ with probability at
    least $1-\delta$, where $\epsilon_r=\epsilon - \frac{r \epsilon}{n} + \frac{r}{n}$.
\end{proof}
